# Supplementary material for: AntiBenford Subgraphs: Unsupervised Anomaly Detection in Financial Networks
Source: arXiv:2205.13426 source file (2022-05-26)
Supplement: Supplementary file 1 [file appendix.tex]

\section{Appendix}

\subsection{Enron Network}

\begin{figure*}[t]
	\centering
	\begin{subfigure}[]{.3\linewidth}
		\centering
		\includegraphics[width=\linewidth]{figs/enron/found0.png}
		\caption{First anomalous subgraph}
		\label{fig:enronfound0}
	\end{subfigure} \quad
	\begin{subfigure}[]{.3\linewidth}
		\centering
		\includegraphics[width=\linewidth]{figs/enron/found1.png}
		\caption{Second anomalous subgraph}
		\label{fig:enronfound1}
	\end{subfigure} \quad
	\begin{subfigure}[]{.3\linewidth}
		\centering
		\includegraphics[width=\linewidth]{figs/enron/found2.png}
		\caption{Third anomalous subgraph}
		\label{fig:enronfound2}
	\end{subfigure}
	\bigskip
	
	\begin{subfigure}[]{.33\linewidth}
		\centering
		\includegraphics[width=\linewidth]{figs/enron/found3.png}
		\caption{Fourth anomalous subgraph}
		\label{fig:enronfound3}
	\end{subfigure} \quad
	\begin{subfigure}[]{.33\linewidth}
		\centering
		\includegraphics[width=\linewidth]{figs/enron/found4.png}
		\caption{Fifth anomalous subgraph}
		\label{fig:enronfound4}
	\end{subfigure}
	
	\caption{Edge weight distribution of five extracted anomalous subgraph comparing to global distribution on Enron network.}
	\label{fig:enron-totalfinding}
\end{figure*}

\subsection{PPI}

\begin{figure}
	\centering
	\begin{subfigure}[]{\columnwidth}
		\centering
		\includegraphics[width=\columnwidth]{figs/ppi/collins_bar.png}
		\caption{Collins network}
		\label{fig:ppicollins}
	\end{subfigure}
	\hfill
	\begin{subfigure}[]{\columnwidth}
		\centering
		\includegraphics[width=\columnwidth]{figs/ppi/gavin_bar.png}
		\caption{Gavin network}
		\label{fig:ppigavin}
	\end{subfigure}
	\caption{Entropy of 6 subgraphs extracted by different peeling heuristics on two PPI networks.}
	\label{fig:ppi_entropy}
\end{figure}

Two yeast protein-protein interaction datasets, Gavin and Collins, are used in this section. Proteins are labeled as non-overlapping clusters, i.e. complex as named in biology, by Munich Information Center for Protein Sequence (MIPS). Besides,  estimation of the reliability of interactions between proteins is available and is included as edge probability attribute. One popular task on such uncertain PPI networks is to mine proteins of the same cluster. Our hypothesis is that, apart from forming dense graph topology, proteins from the same complex are likely to have similar edge probabilities between each other. If our assumption holds, local edge probability histograms of a complex should have large $\chi ^2$ statistics comparing to the global histogram. 

To testify our hypothesis, we implement our algorithm, as well as unweighted and weighted dense subgraph heuristics on two networks. Edge probability is treated as edge attribute in our algorithm. Besides, edge weight is set to 1 for unweighted greedy peeling, and set to the probability of each edge for weighted version. For each network, we apply the peeling process six times (remove nodes of extracted subgraph before next peeling) to generate top 6 subgraphs, and evaluate the purity of subgraph by calculating the entropy according to MIPS labels each subgraph contains. Given each label $k$ its proportion in all labels of the subgraph $P_k$, entropy is defined as $Entropy = -\sum_k (P_k*\log P_k)$. Intuitively, the entropy would be 0 if all nodes in the subgraph are from one complex, and gets larger if node has more different labels. Entropy of subgraphs generated by different methods are reported in Figure~\ref{fig:ppi_entropy}. We observe the entropy of our algorithm remains the lowest among all top six results. Note that the average size of the subgraphs found by our algorithm is 28.3 for Collins and 5.3 for Gavin, while the average size of complex labeled by MIPS is 12.5 so our findings are not trivial. This shows our algorithm is capable of precisely finding complex on uncertain PPI networks, and performs better compare to existing dense subgraph heuristics.

\subsection{Slashdot}

In this section we apply our algorithm on a social relation network to find abnormal subgraphs. Slashdot network is a graph of website users with edges tagging the relationship (friend or foe) between users. Frequency distribution of size 3 motifs comparing to configuration model is shown in Figure~\ref{fig:slashcompare}. One interesting result we find is by contrasting motif 7 and 10, result subgraph is visualized in Figure~\ref{fig:slashgraph}. Remind that social networks commonly share triadic closure, i.e. a friend of my friend is tend to be my friend, and extension can be an enemy of my enemy is my friend. However this property is broken among some triangles in this subgraph, where relations of "all enemies" and "two friends and one enemy" exist.

\makebox[0pt][l]{%
	\begin{minipage}{\columnwidth}
		\centering
		\includegraphics[width=\columnwidth]{figs/slashdot/random_compare.png}
		\captionof{figure}{distributions of motifs of size 3 of Slashdot and configuration model}
		\label{fig:slashcompare}
	\end{minipage}
}

\makebox[0pt][l]{%
	\begin{minipage}{\columnwidth}
		\centering
		\includegraphics[width=\columnwidth]{figs/slashdot/contrast_7_10_i=0shape.png}
		\captionof{figure}{Subgraph extracted by contrasting motif 7 and 10 on Slashdot.}
		\label{fig:slashgraph}
	\end{minipage}
}
